# Supplementary material for: EResFD: Rediscovery of the Effectiveness of Standard Convolution for Lightweight Face Detection
Source: arXiv:2204.01209 source file (2023-11-02)
Supplement: Supplementary file 1 [file Appendix.tex]

\newpage{}

\section{Implementaion details}
\subsection{Anchor Settings}  As shown in Table \ref{tab:anchor_setting}, anchors whose sizes are ranged from 16 to 512 are assigned from detection layers from D1 to D6, following \cite{s3fd}. Anchor width ratio to the height is set to 1:1.25. 

\input{table_appendix_anchor}

\subsection{Training}
During training, we adopt data pre-processing steps, augmentation strategies, and loss functions  used in \cite{s3fd}. Specifically, we used color distortion by by changing hue, saturation, value (brightness) of an image. Also, for generating various scales of faces, zoom-in and out operation are applied to image along with its face bounding boxes. Consequently, the resultant image is resized to 640 $\times$ 640 after horizontal flipping. Also, max-out background label~\cite{s3fd} is applied on D1 detection head for reducing false positives with regard to small faces. We also employed multi-task loss, where both classification and regression loss are normalized by number of positive anchors. We set balancing parameter between classification loss and regression loss as 1.

With regard to optimization hyper-parameters, we used ADAM~\cite{kingma2014adam} optimizer with initial learning rate 0.001, weight decay 5e-4, and batch size 32. The maximum number of iterations is 330k and learning rate is decayed at [250k, 300k, 320k] by 0.1.
% OHNM?
% \begin{itemize}
%     \item Color distort: random distortion to the image by changing hue, saturation, value (brightness).
%     \item Zoom-in/out augmentation: For generating various scales of faces, zoom-in and out operation~\cite{s3fd} are applied to image along with its face bounding boxes.
%     \item Horizontal flip:
% \end{itemize}
% Input size
% random distort (hsv, with 50% p)

\subsection{Evaluation} For evaluation on WIDER FACE, we employed flip and multi-scale testing~\cite{s3fd}, where all these predictions are merged by Box voting~\cite{gidaris2015object} with IOU threshold at 0.3. 
In case of using RetinaFace framework~\cite{deng2019retinaface}, we used single-scale testing where original image size is maintained.
% AFLW NME 실험 세팅?
% 실험 셋팅 설명
% S3FD trianing & eval 세팅?
% RetinaFace training & eval 세팅?

\section{Stem Modification}
\input{table3_stemlayer_acc} % stem layer에 대한 실험과 설명을 추가할지 고민.. (위에서 이미 전체 latecy가 확인되기에)
% We also compare the stem layer
In Table \ref{table:stemlayer_modification_performance}, we compare detection performance depending on the design of stem layer. It is worth notable that our proposed stem layer requires much more reduced computational costs with significantly improved detection accuracy scores compared to that of ResNet.

\section{SepFPN}
 In Figure \ref{fig:sepfpn_p3_p4}, we visualize the architecture of variations for our proposed SepFPN, where its separation position is varied from P3 to P4. 
\begin{figure}[t]
    \centering
    \begin{subfigure}[t]{0.5\linewidth}
        \includegraphics[width=1.1\linewidth]{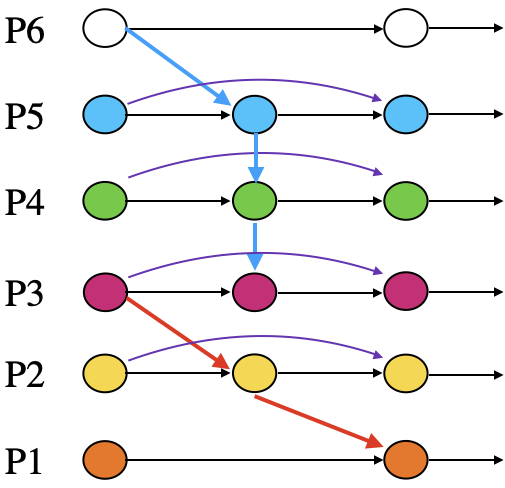}
        \centering
    \subcaption{Separation position: P3}
    \vspace{3mm}
    \end{subfigure}
    \begin{subfigure}[t]{0.5\linewidth}
        \includegraphics[width=1.1\linewidth]{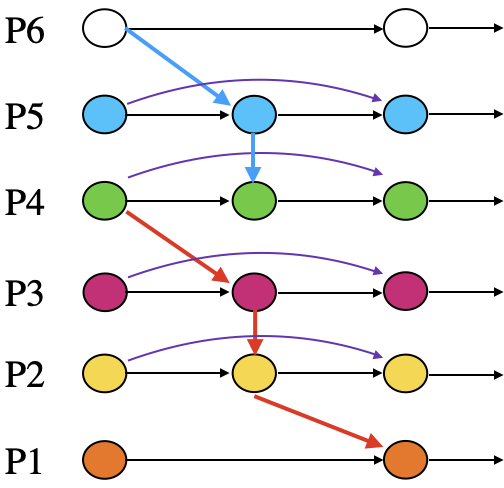}
        \centering
    \subcaption{Separation position: P4}
    \end{subfigure}
    \caption{Architectures of SepFPN with various separation positions (P3, P4).}
    \label{fig:sepfpn_p3_p4}
\end{figure}
